# Supplementary material for: Beyond FVD: Enhanced Evaluation Metrics for Video Generation Quality
Source: arXiv:2410.05203 source file (2024-10-08)
Supplement: Supplementary file 1 [file metric_guidelines.tex]

% will be added to our webpage.
% \section{Guideline for Accurately Evaluating Video Distribution Distance\label{sec:metric_guideline}}
% To ensure reliable evaluation of video distribution distance, please consider the following guidelines:
% \begin{enumerate}
%     \item 
%     \textbf{Avoid averaging distributional metric distances in minibatches. } Distributional metrics necessitate comprehensive sample sizes to converge and precisely capture the underlying distribution. Recognizing that infinite data is theoretically required for accurate distance evaluation, it is recommended to compute metric distances on the entire dataset, ensuring reliable and robust assessments.
%     \item 
%     \textbf{Extract features in minibatches. } Due to GPU memory constraints, processing entire datasets at once may not be feasible. To address this, features can be extracted in minibatches, saved, and then utilized in their entirety during evaluation.
%     \item 
%     \textbf{Assert consistence video settings. }Verify identical video settings, such as frame resolution, frame rate, and video length, for both distributions. Also, confirm consistent settings when comparing with other studies.
%     \item
%     \textbf{Report the ground-truth baseline. }Report the distribution distance between the ground truth training and testing sets. This provides a reference point for evaluating generated video quality against the empirical dataset distance.
% \end{enumerate}
